# Supplementary material for: Demonstration of Machine Learning-assisted real-time noise regression in gravitational wave detectors
Source: arXiv:2306.11366 source file (2023-06-20)
Supplement: Supplementary file 1 [file sec-appendix-injections.tex]

%\section{Detailes of the MDC injections}\label{sec-mdc-appendix}

% \begin{figure*}
%     \centering
%     \includegraphics[scale=0.2]{figures/injection_mass_distribution.pdf}
%     \caption{Caption}
%     \label{fig:inj-masses}
% \end{figure*}

% \begin{figure*}
%     \centering
%     \includegraphics[scale=0.12]{figures/injection_sky_positions.pdf}
%     \includegraphics[scale=0.12]{figures/injection_temporal_distribution.pdf}
%     \caption{Caption}
%     \label{fig:inj-skypositions}
% \end{figure*}
